# Supplementary material for: On Pursuit of Designing Multi-modal Transformer for Video Grounding
Source: arXiv:2109.06085 source file (2022-04-11)
Supplement: Supplementary file 1 [file figVisUmap.tex]

\begin{figure*}[t]
	\centering
	\includegraphics[width=\textwidth]{figs/embedUMAP.pdf}
	\caption{\small UMAP visualizations of video feature for three different embedding ways. Green points represent action snippets and gray points denote background snippets. Our Cubic Embedding achieves a more separable feature distribution compared to the others.}
	\label{fig:visumap}
\end{figure*}
