# Supplementary material for: On Pursuit of Designing Multi-modal Transformer for Video Grounding
Source: arXiv:2109.06085 source file (2022-04-11)
Supplement: Supplementary file 2 [file figVisWordSelf.tex]

\begin{figure}[!h]
	\centering
	\includegraphics[width=0.3\textwidth]{figs/wordSelfAtten.pdf}
	\vspace{-3pt}
	\caption{\small Word Self Attention in Language Encoder.}
	\label{fig:wordSelfAtten}
\end{figure}
